# Supplementary material for: Quantifying Feature Space Universality Across Large Language Models via Sparse Autoencoders
Source: arXiv:2410.06981 source file (2025-05-21)
Supplement: Supplementary file 1 [file appendix_pt3.tex]

\section{Novelty and Purpose of Studying Feature Space Universality}
\label{app:}

In contrast to previous papers, we are applying representational similarity on features in weight space, instead of on input data samples in activation space. This allows us to assess if we can use features, not input samples, to determine if representations are the same across models.

The main research question we are tackling is: are the relationships among SAE features similar even if the features appear different? As an analogy, consider three points [1, 2, 3] on a right triangle. We can think of each point like a feature. One model may label these points as [A, B, C], and another model may label these points as [X, Y, Z]. However, these points are not ordered as columns in a matrix, so we may find them in the order of [B, C, A] and [Z, X, Y]. But if we rearrange them together into “close enough” pairs, we may figure out what points they correspond to on the right triangle, and then measure if the relationship among them- the right triangle- is also similar. Moreover, high similarity scores for our measures do not require these features to correspond to the exact same right triangle; rather, just that the relationship among these features forms a right triangle. We refer to these relationships and their points as being “analogous” to one another, and it is possible they may be similar under transformation.

This is not always the case, because model A may learn the features that activate on {dog, cat, mouse} tokens and model B may learn features that seemingly also activate similarly on {dog, cat, mouse} tokens. However, it is possible that the {dog, cat, mouse} features learned by these two models belong to two very different representations. 

This is a different research question than the ones studied by previous papers, as they did not measure the relationships among features, but among input data samples that are already known to correspond to the “same point” in input data space. 

Previous Papers: To elaborate, SVCCA compares two matrices by their matched row samples to assess the similarities of their column spaces. The rows are samples from each column space. In previous works, SVCCA was measured by taking these samples using input data samples’ activations. For instance, both models A and B take in the input sample “Eliza went swimming” from the same point in input space, so we can match the rows of the activations for that input sample. The columns are the LLM activation space dimensions.

How our Method Differs: In contrast to previous works, we are not measuring LLM activation spaces, but SAE weight spaces, which learn features not explicitly present in LLM space. Thus, the rows are SAE feature weights, not input samples. Unlike previous works, it is not immediately obvious which features correspond to “analogous” points that collectively form similar representations. To solve this, we estimate which features can pair with another using activation correlation, and compare thousands of feature pairs. While few pairings are “good”, multiple good pairings are possible.

Thus, previous research papers did not check if the features learned by models belong to points that form similar representations. In other words, even though models / SAEs may label these features with different vector values, they may be “mappable” under permutation and rotational invariance. This is novel as it would introduce a new perspective to thinking about how different models represent features, and how feature decomposition methods like SAEs learn these features. We find evidence that suggests this new perspective should be taken into account for future research.

Another contribution of this paper is to measure how well feature decomposition methods, like SAEs, obtain features that have similar relations among each other across models. Our results suggest that even if SAEs across different models learn different features, there may be “analogous transformations” between their feature representations. Still, these results are affected by how SAEs may not always learn the same features, and may not learn “good” features, which means similar pairings between features may not always be found. This motivates future work to develop techniques that allow better, more consistent features to be learned. 

\section{Applications}
\label{app:}

we stated that the main aim of the paper is to measure if the subset of features learned by SAEs form “analogous representations across models”. The purpose of doing this is to better understand: 1) what types of features are learned by LLMs, and 2) how well these features are captured via decomposition methods like SAEs.

If models are learning features that belong to “analogous representations”, it suggests that there is universality in terms of how their learned features relate to one another. This would motivate further work that aims to harness this universality so that methods which manipulate features in one model can be transferred to another model, possibly through learned transformations between models. This is similar to work which learned affine mappings between image to text models \citep{merullo2023linearlymappingimagetext}. Our work provides possible insight clues into how these mappings work.

For mechanistic interpretability, we want to find universal principles that models share. This is because AI models evolve fast, so we want interpretability discoveries to not just give information on a narrow subset of models, but on new models as well. Currently, much work in mechanistic interpretability relies on looking for specific features within a sample of models. However, in order for these findings to generalize, it is more potent to look for underlying principles, rather than specific discoveries restricted within some models. 

Additionally, if these are shared “platonic” spaces that models work under, this would motivate research that modifies concepts in this “shared space” such that techniques can work across models, rather than applying techniques restricted to specific models. Currently, techniques like steering vectors, which rely on relations between features, have been found to work within models. However, each steering vector is very model-specific; thus, finding universal steering vectors would be immensely useful.

One motivation for our work stemmed from extending Anthropic’s findings about SAE feature spaces, specifically on their work about SAE universality \citep{bricken2023monosemanticity} and feature spaces \citep{templeton2024scaling}. Previously, Anthropic only conducted work on individual feature similarity across toy models. We extend this work to study similarities across more than just toy models.
